# Supplementary material for: Kernel Distributionally Robust Optimization
Source: arXiv:2006.06981 source file (2021-02-27)
Supplement: Supplementary file 1 [file additional.tex]

\subsection{Prove that the constraint is convex}
\begin{proof}
    Let $P_1, P_2\in \mathcal C$, and let  $P = t P_1+(1-t)P_2$, where $t\in[0,1]$. It suffices to show $P\in\mathcal C$ for any choices of $P_1, P_2, t$. Let $\mu_P = \int\phi(x)dP(x)$, we have
    \begin{multline*}
     \|\mu_P - \hat\mu\|_\rkhs= \|t\mu_{P_1} - t\hat\mu +(1-t)\mu_{P_2} - (1-t)\hat\mu\|_\rkhs\\
     \leq \|t\mu_{P_1} - t\hat\mu \|_\rkhs+\|(1-t)\mu_{P_2} - (1-t)\hat\mu\|_\rkhs\\
     \leq t\epsilon + (1-t)\epsilon = \epsilon.
     \end{multline*}
    Hence, $P\in\mathcal C$.
\end{proof}

\subsection{Lemma~\ref{thm:wc_dist_supp} worst-case distribution}
\begin{proof}
    Suppose $\genset$ is a generating class of $\mathcal P$.
    Let us consider the following program
    $$
    \begin{opt1}
        (P'):=\MAXST{P\in \genset,\mu\in \mathcal C}{\int l \ dP}
        {\int{\phi}{\ dP} = \mu},
    \end{opt1}     
    $$
    since $\mathrm{mix}(\genset) = \mathcal P$, the dual of (P') is simply (D). 
    $\genset\cap\mathcal K \neq \emptyset$ implies that the set 
    $$
    \genset_{\mathcal C}:=\{\tau\colon \mu_\tau \in \mathcal C, \tau\in\genset\}
    $$
    has nonempty interior.\jz{or relative interior?} 
    Then (P') is strictly feasible. Let $\tau^*\in\genset$ be the optimal solution of (P'). By strong duality,
    $$
    \pip{l}{\tau^*} = (D'') = (D) = (P),
    $$
    i.e., there exists a measure $\tau^*\in\genset$ that attains the worst-case risk.
\end{proof}

\subsection{$\epsilon$-metric ball case: Worst-case distribution \ref{thm:wc_dist}}
\begin{proof}
    Because $\mathcal C=\{\mu\colon\|\mu - \hat\mu\|_\rkhs\leq \epsilon\}$,
    the set $\genset\cap\mathcal K \neq \emptyset$ at least contains one element $\hat P$.
    Applying \ref{thm:wc_dist_supp}, we obtain the result.
    
    The seond claim is similar.
\end{proof}
From the proof, it is clear that the statement of the reuslt is not true for distributions supported on fewer than $N$ points --- indeed, if we replace $\genset$ with $\mathbb T_{N-1}$, the primal problem might not be feasible and we can not guarantee strong duality in such cases. 
An alternatively proof for a similar result using measure theoretical techniques can be found in \cite{parysDistributionallyRobustControl2015}, Theorem~3.3.

---
Let us consider the well known conditional value-at-risk as a special case of our applciation. \jz{use the simple dual rep. don't use this}
\begin{example}
        (Duchi's form and worst-case conditional value-at-risk)
\begin{multline*}
\min_x\sup_P \mathrm{CVaR}_{\epsilon}(l(x,w)) = \min_x\sup_P\inf_t\{t + \frac1\epsilon\mathbb E\left[l(x,w) - t\right]^+\}\\
= \min_x\inf_t\{t + \sup_P\frac1\epsilon\mathbb E\left[l(x,w) - t\right]^+\} \\
=\inf_t\{t + \min_x\sup_P\frac1\epsilon\mathbb E\left[l(x,w) - t\right]^+\}
\end{multline*}
The function $\mathbb E\left[l(x,w) - t\right]^+$ is convex in $t$. It is convex in $x$ if $l(x,w)$ is convex in $x$. Inspecting the inner min-max problem, we see that this reduces to solving ~\eqref{eq:kdro}. This was extensively studied in operations research such as in \cite{zymlerDistributionallyRobustJoint2013}, Parys, Shapiro risk measure. The authors of [duchi] also discussed using RKHS with this risk measure.
Specifically, they used the approximation
$$
\mathbb E\left[l(x,w) - t\right]^+\approx \sup_{h:\mathcal X\to[0,1]}\mathbb E h(w)(l(x,w) - t)
$$
i.e., using a certain class of functions to approximate the characteristic function $\left[\cdot \right]^+$. They consider the case where $h$ belongs to an RKHS.
\end{example}

%%%%%%%%discuss reduction to krr
Frist, we establish trivial connection between our formulation and kernel-based learning, whose robustness is well-known due to \cite{christmannRobustnessPropertiesConvex, christmannConsistencyRobustnessKernelbased2007}. The proof is by simply constraining the cost funciton in ~\eqref{eq:conic_dual} to be in the RKHS and hence trivial.

\subsection{choquet and rkhs}
If we consider the loss function to be an RKHS function, we obtain the following result that reveals the conneciton between Choquet represetnation and kernel method.
\begin{proof}
        \input{draft/pf/choquet_rkhs.Rmd}
\end{proof}

\section{ball on the ground example}
\begin{figure}[b!]
	\centering
	\includegraphics[width=\columnwidth]{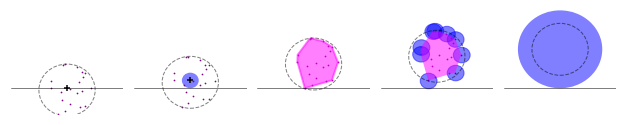}
	\caption{Imagine an hyperthetical scenario that we want to simulate a ball on the ground. However, due to reasons such as perception error, we do not known its size accurately, but only an upper bound as in (e). We can simply place the ball to make sure it's above the ground in the \emph{worst-case} scenario. Suppose, to take a data driven approach, we are given samples known to lie inside the ball. We can optionally ensure the mean of samples is above the floor (a), or add to it some margin (b), ensure all samples above the floow (c), or ensure margin around all samples (d). The intuition of (e) is that of the \emph{classical robust optimization} and (a) that of sample average approximation. By properly applying geometric intuition with data, we may improve the performance and strike a balance between performance and robustness. This paper will combine such geometric insights with RKHS theory.}
	\label{fig:ball}
\end{figure}
